# Supplementary material for: Evidence for the spin-0 nature of the Higgs boson using ATLAS data
Source: arXiv:1307.1432 source file (2013-07-04)
Supplement: Supplementary file 1 [file CombAppendix.tex]

The material included here below is meant to be approved as Auxilliary material.

\begin{figure*}[htb]
 \centering
 \includegraphics[width=\textwidth]{figures/hgg/Hgg_spin_decorrelation}
 \caption{
   This figure displays information on the possible existence of correlation between the
   observables \costs\ and \mgg\ in the background events, as
   observed from the data sidebands ($105\gev < \mgg < 122\gev$ and $130\gev < \mgg < 160\gev$). The variable shown is the ``pull'',
   defined as the difference between the number of observed events ($n^{\mathrm{obs}}$) and the number of
   expected events ($n^{\mathrm{exp}}$) in the case of no correlation, divided by
   its statistical uncertainty. The quantity $n^{\mathrm{exp}}$ is computed from
   the product of the two observed marginal distributions, each obtained
   by projecting the two-dimensional distribution on either of the two
   observables. The plot on the left shows the values of the pull in bins of
   $\costs \times \mgg = 0.1 \times 1\gev$. The plot on the right shows its
   distribution, overlaid with a Gaussian distribution with 0 mean and standard deviation of 1. The
   compatibility between the histogram and the curve, expressed in terms
   of the $\chi^2$ divided by the number of degrees of freedom (ndf), and of
   the confidence level CL, indicates that the data in the sideband region are
   consistent with the absence of correlations between \costs\ and
   \mgg.
 }
 \label{fig:Hgg_spin_decorrelation}
\end{figure*}

\clearpage

\begin{figure*}[htbp]
 \centering
 \includegraphics[width=\columnwidth]{figures/hgg/Hgg_spin_decorrelation_ratio}
 \caption{
   The ratio $f'(\costs)/f(\costs)$ of two different estimates of the 
   background \costs\ distributions in the signal region ($122\gev < \mgg < 130\gev$). 
   The distribution in the denominator, $f(\costs)$, is that used 
   in the spin analysis, and it is given by the normalised distribution of \costs, 
   built from all events in the sidebands ($105\gev < \mgg < 122\gev$ and $130\gev < \mgg < 160\gev$). The distribution in the numerator, $f'(\costs)$,
   is obtained from the normalised estimate of the number of background events in each
   \costs\ bin in the signal region, through a fit of an analytical function to the observed \mgg\
   data in the sidebands. 
   This procedure treats all \costs\ bins independently of each other,
   therefore it is sensitive to possible correlations between \mgg\ and \costs.
   The compatibility of the ratio $f'(\costs)/f(\costs)$ with unity implies that no
   significant correlation between \mgg\ and \costs, within the
   current precision, is observed in the data.
   The orange and blue bands correspond, respectively, to the statistical
   uncertainty from the sidebands and the total uncertainty on the
   background model. The vertical bars on the solid dots reflect the statistical uncertainty
   of the fit.
 }
 \label{fig:Hgg_spin_decorrelation_ratio}
\end{figure*}

\begin{figure*}[htbp]
  \centering
  \includegraphics[width=\columnwidth]{figures/hgg/Hgg_spin_LLR_ggF}
  \caption{
    Expected distributions of the test statistics \mbox{$q=\log({\cal L}(0^+)/{\cal L}(2^+))$} for the spin-0 and
    spin-2 (produced by gluon fusion) hypotheses. The observed value is indicated by a vertical line. The
    coloured areas correspond to the integrals of the expected
    distributions used to compute the $p$-values for the rejection of each
    hypothesis.
  }
  \label{fig:Hgg_spin_LLR_ggF}
\end{figure*}

\begin{figure*}[htbp]
\centering
\subfigure[\label{fig:exclA}]{\includegraphics[width=0.4\textwidth]{figures/hcomb/comb_llr_v2.pdf}}
\subfigure[]{\includegraphics[width=0.4\textwidth]{figures/hcomb/comb_llr_v2_2band}}
 \caption{\label{fig:excl} Expected and observed ratio of the test statistics $q$, defined as \mbox{$q=\log({\cal L}(0^+)/{\cal L}(2^+))$}, 
for the combination of channels as a function of the fraction of the $q\bar{q}$ spin-2 production mechanism. The green and yellow bands represent, respectively, the one and two standard deviation bands for the
  \spinzero\ (a) and for the \spintwo\ (b) hypotheses.}
\end{figure*}

%\clearpage

\begin{figure*}[!htpb]
\centering
\subfigure[]{\includegraphics[height=0.33\textwidth]{figures/hcomb/comb_rpl_100gg_log}}
\subfigure[]{\includegraphics[height=0.33\textwidth]{figures/hcomb/comb_rpl_75gg_log}}
\subfigure[]{\includegraphics[height=0.33\textwidth]{figures/hcomb/comb_rpl_50gg_log}}
\subfigure[]{\includegraphics[height=0.33\textwidth]{figures/hcomb/comb_rpl_25gg_log}}
\subfigure[]{\includegraphics[height=0.33\textwidth]{figures/hcomb/comb_rpl_00gg_log}}

 \caption{Expected distributions of \mbox{$q=\log({\cal L}(0^+)/{\cal L}(2^+))$}, the logarithm of the ratio of profiled likelihoods under the spin-0 and 
spin-2 hypotheses, in the  presence of spin-0 (blue distributions) or spin-2 (red distributions) signals for various fractions of \qqbar\ production 
of the spin-2 signal (\fqq): (a) $\fqq = 0\%$; (b) $\fqq = 25\%$; (c) $\fqq = 50\%$; (d) $\fqq = 75\%$; (e) $\fqq = 100\%$.  
The observed values are indicated by a vertical line.  The coloured areas correspond to the integrals of the expected distributions 
up to the observed values and are used to compute the $p_0$-values for the rejection of each hypothesis.}
\end{figure*}

\begin{figure*}[!hbp]
\centering
 \subfigure[\hgg]{\includegraphics[height=0.4\textwidth]{figures/hcomb/gammagamma_fqq}}
 \subfigure[\hzz]{\includegraphics[height=0.4\textwidth]{figures/hcomb/zz_fqq}}
\subfigure[\hww]{ \includegraphics[height=0.4\textwidth]{figures/hcomb/ww_fqq}}
 \caption{\label{fig:qqscan} Observed values of the test statistic \mbox{$q=\log({\cal L}(0^+)/{\cal L}(2^+))$}  
(black solid line) as a function of the fraction of \qqbar\ production of the spin-2 state \fqq\ for the \hgg\ (a), \hzz\ (b) and \hww\ (c) channels. 
The blue and red dashed lines indicate the positions of the median expected values of the sampling distributions for the spin-0 and spin-2 signals, respectively, obtained from pseudo-experiments. 
The green and yellow bands correspond, respectively, to one and two standard deviations around the spin-0 median curve.}
\end{figure*}

\begin{table*}
\caption{\label{tab:resMu1}Expected and observed $p_0$-values for the \spinzero\ and \spintwo\ hypotheses as a function of the fraction \fqq\ of the $q\bar{q}$ spin-2 production mechanism.  The values are calculated for the combination of the \hgg, \hzz\ and \hww\ channels. The pseudo-experiments corresponding to the $J^P = 0^+$ hypothesis are generated following the Standard Model predictions for the signal strength in each channel while for the \spintwo\ hypothesis 
the signal strengths fitted to the data are used.}
\vspace{3mm}
\centering

\resizebox{\textwidth}{!}{
\begin{tabular}{c||c|c||c|c||c}
\hline\hline
\multirow{2}{*}{\fqq} & spin-2 assumed & spin-0 assumed & \multirow{2}{*}{Obs. $p_0(\spinzero)$} & \multirow{2}{*}{Obs. $p_0(\spintwo)$} & \multirow{2}{*}{$\CLs (\spintwo)$} \\
   & Exp. $p_0(\spinzero)$ & Exp. $p_0(\spintwo)$ & & & \\
\hline
100\% & $1.1\cdot 10^{-2}$ & $4.2\cdot 10^{-3}$ & 0.98 & $1.6\cdot 10^{-6}$ & $7.8\cdot 10^{-5}$ \\
75\% & $2.0\cdot 10^{-2}$ & $1.1\cdot 10^{-2}$ & 0.96 & $3.2\cdot 10^{-5}$ & $8.1\cdot 10^{-4}$ \\
50\% & $2.1\cdot 10^{-2}$ & $2.1\cdot 10^{-2}$ & 0.97 & $8.6\cdot 10^{-5}$ & $2.8\cdot 10^{-3}$ \\
25\% & $9.5\cdot 10^{-3}$ & $1.9\cdot 10^{-2}$ & 0.97 & $0.9\cdot 10^{-4}$ & $3.3\cdot 10^{-3}$ \\
0\% & $2.1\cdot 10^{-3}$ & $1.0\cdot 10^{-2}$ & 0.95 & $1.5\cdot 10^{-4}$ & $2.9\cdot 10^{-3}$ \\
\hline\hline
\end{tabular}}

\end{table*}

\clearpage 

\begin{figure*}[!hbp]
  \centering
  \subfigure{\includegraphics[width=0.23\textwidth]{figures/hww/dphill}}
    \subfigure{\includegraphics[width=0.23\textwidth]{figures/hww/dphill_spin2}}
  \subfigure{\includegraphics[width=0.23\textwidth]{figures/hww/mll}}
    \subfigure{\includegraphics[width=0.23\textwidth]{figures/hww/mll_spin2}}
  \subfigure{\includegraphics[width=0.23\textwidth]{figures/hww/ptll}}
  \subfigure{\includegraphics[width=0.23\textwidth]{figures/hww/ptll_spin2}}  
  \subfigure{\includegraphics[width=0.23\textwidth]{figures/hww/met}}
    \subfigure{\includegraphics[width=0.23\textwidth]{figures/hww/met_spin2}}
  \caption{\label{fig:shapes} Distributions of \dphill, \mll, \ptll, and \metrel\ for the \hww\ channel for different spin hypotheses after requiring two opposite-charge leptons,  $\met > 20$~GeV, and zero jets. The
    definitions of these quantities are discussed in the text. The
    distributions are normalised to unit area.}
\end{figure*}

\begin{figure*}[!hbp]
\centering
\subfigure{\includegraphics[width=0.4\textwidth]{figures/hww/emme_CutTopoDPhill_0jet_Ptll_nb_mh125_lin_newcolor}}
\subfigure{\includegraphics[width=0.4\textwidth]{figures/hww/emme_CutTopoDPhill_0jet_MT_nb_mh125_lin_newcolor}}
\vspace*{-0.5cm}
\caption{\ptll\ and \mT\ distributions in the signal region. %The lepton flavours are combined.
    The signal shown is for $m_{H} = 125\GeV$ and the \spinzero\ hypothesis. 
    The shaded area represents the uncertainty on the signal and background yields from statistical, experimental, and theoretical sources.
  }
\label{fig:SRInputVars}
\end{figure*}

\begin{figure*}[!hbp]
\centering
\subfigure{\includegraphics[width=0.4\textwidth]{figures/hww/emme_CutTopoDPhill_0jet_BDT0_fine_mh125_lin_newcolor}}
\subfigure{\includegraphics[width=0.4\textwidth]{figures/hww/emme_CutTopoDPhill_0jet_BDT2_fine_mh125_lin_newcolor}}
\subfigure{\includegraphics[width=0.4\textwidth]{figures/hww/emme_CutTopoDPhill_0jet_BDT7_fine_mh125_lin_newcolor}}
\subfigure{\includegraphics[width=0.4\textwidth]{figures/hww/emme_CutTopoDPhill_0jet_BDT8_fine_mh125_lin_newcolor}}
\vspace*{-0.5cm}
\caption{Distributions of the BDT output in the signal region. The distribution obtained in data 
is compared to the sum of the expected backgrounds and \spinzero signal hypothesis. BDT(0+) refers to the BDT optimized for \spinzero\ separation from 
the background, while the second BDT, BDT(2+,\fqq = 25\%), BDT(1-) or BDT(1+), is used to separate the alternative spin 
hypothesis (\spintwo, \spinonem\ or \spinonep) from the background. The signal is scaled to the 
SM \spinzero\ cross section. The shaded area represents the uncertainty on the signal and background yields from statistical, 
experimental, and theoretical sources.
  }
\label{fig:SRBDToutput}
\end{figure*}

\clearpage 

\begin{figure*}
\centering
\subfigure{\includegraphics[width=0.4\textwidth]{figures/hww/125_MVAOutput0_20bins_0jet_emu_all_shape}}
\subfigure{\includegraphics[width=0.4\textwidth]{figures/hww/125_MVAOutput2_20bins_0jet_emu_all_shape}}
\caption{BDT output distributions in the signal region, showing the
  shape differences between the \spinzero\ and \spintwo\ (\fqqf{25}) signals and the
  backgrounds, for the BDT trained with \spinzero\ signal (left) and
  trained with \spintwo\ signal (right). The distributions are normalised to unit area.}
\label{fig:SRBDTShapes}
\end{figure*}

\begin{figure*}[!hbp]
  \centering
\subfigure{\includegraphics[width=0.4\textwidth]{figures/hww/spin2p_25qq_allsys_strategy1_high_samplings_newstyle}}
\subfigure{\includegraphics[width=0.4\textwidth]{figures/hww/spin2p_100qq_allsys_strategy1_withlog_high_samplings_newstyle}}
\subfigure{\includegraphics[width=0.4\textwidth]{figures/hww/spin1m_allsys_strategy1_high_samplings_newstyle}}
\subfigure{\includegraphics[width=0.4\textwidth]{figures/hww/spin1p_allsys_strategy1_high_samplings_newstyle}}
\caption{\label{fig:result_allfrac} 
Top: Distributions of the test statistics, defined as \mbox{$q=\log({\cal L}(0^+)/{\cal L}(2^+))$}, 
for \spinzero (blue) and \spintwo (red) as well as the observed value (solid line) for the two
different \spintwo\ production working points:  \fqqf{25} (left) and \fqqf{100} (right). 
 Bottom: Test statistics distributions for \spinzero (blue) and \spinonem (left plot, red)
 or \spinonep (right plot, red) as well as the observed value (solid line).
The median of each of the distributions is indicated by a
dashed line. The shaded areas correspond to the observed
$p_0$-values. The distributions are normalised to unit area.} 
\end{figure*}
